# Supplementary material for: Online Regenerator Placement
Source: arXiv:1309.0195 source file (2013-09-01)
Supplement: Supplementary file 1 [file appendix.tex]

\newpage
\appendix

\noindent{{\Large \textbf{Appendices}}}
